# Supplementary material for: Spin caloritronics in a CrBr$_3$-based magnetic van der Waals heterostructure
Source: arXiv:2005.03561 ancillary file (2020-05-07)
Supplement: Supplementary file 1 [file supporting_information.pdf]

# Supporting Information: Spin caloritronics in a $CrBr_3$ based magnetic van der Waals heterostructure

Tian Liu,* Julian Peiro,† Dennis K. de Wal, Johannes C. Leutenantsmeyer, Marcos H.D. Guimarães, and Bart J. van Wees
*Zernike Institute for Advanced Materials, Nijenborgh 4, 9747 AG Groningen, The Netherlands*

(Dated: May 6, 2020)

**Contents**

I. Fabrication methods 2
A. Source of the material 2
B. Preparation for the substrate and metal contacts deposition 2
C. Dry transfer in inert atmosphere 2

II. Atomic Force Microscopy 2

III. Magnetic Circular Dichroism measurement 2

IV. Electrical measurement 3
A. Electrical characterization 3
B. Local signal 3
C. Non-local first harmonic signals 3
D. Offset of the non-local second harmonics 3
E. Methods for nl-ADMR measurements and their fitting 3

V. Spin signal measured at different contact pairs 4

VI. Temperature dependence of spin Seebeck signal 4

VII. Finite element heat distribution simulation 5
A. Geometry, conditions and parameters 6
B. Simulation and results 6
1. Temperature profiles in the $CrBr_3$ layer 7
2. Temperature gradients profiles in the $CrBr_3$ layer 8
3. Temperature gradients in the platinum detector and at the interface 9
C. Estimation of a spin Seebeck coefficient 9

VIII. An overview of bulk, interface and proximity spin-caloritronics effects 10
A. Seebeck effect 10
B. Spin Nernst Magnetoresistance 10
C. Proximity Anomalous Nernst Effect 11
1. Relevance of a proximity induced magnetism in platinum 11
2. Contribution of the anomalous Nernst effect 11
3. Revealing the anomalous Nernst effect induced by horizontal heat flow 12
D. Extraction of the spin Seebeck contribution 13

References 14

* tian.liu@rug.nl; Contributed equally to this work
† Contributed equally to this work

# I. Fabrication methods

## A. Source of the material

$CrBr_3$ and hBN crystals are provided by a commercial company HQgraphene, the same batch with the paper "Magnon-assisted tunnelling in van der Waals heterostructures based on $CrBr_3$"[1].

## B. Preparation for the substrate and metal contacts deposition

The bottom hBN flake is exfoliated on a $SiO_2$(285 nm)/Si substrate. A first e-beam lithography (EBL) step is used to define a PMMA mask layer for patterning the Au/Ti leads of the device. An adhesion layer of 5 nm of Ti followed by 50 nm of Au are then deposited by e-beam evaporation, and lifted-off. Then a second EBL step pattern a new PMMA layer for the Pt electrodes. A CF4-plasma etching allows to dig into the hBN before deposition of the 6 nm of Pt in order to embed the electrode so that the height difference between the top of the Pt contact and the surrounding hBN is reduced. Ideally, a flat surface would enhance the encapsulation quality.

## C. Dry transfer in inert atmosphere

We use a standard dry transfer technique for vdW stacking[2]. The transfer (stacking) stage is built in an glove box filled with inert gas Argon, with water and oxygen concentrations below 0.5 ppm. The transfer steps are the following: first a top hBN layer is picked up by a polydimethylsiloxane/polycarbonate (PDMS/PC) stamp; then a thin $CrBr_3$ flake is picked up by the top hBN layer attached to the stamp, with careful alignment; finally the hBN/$CrBr_3$ structure is deposited onto a prepatterned Pt/hBN substrate. The temperature used for picking up flakes ranges from 90 °C to 110 °C. We use 190 °C to melt the PC film in the last step. After fabricating the van der Waals stack, we dissolve the PC film in Chloroform for 5 mins.

# II. Atomic Force Microscopy

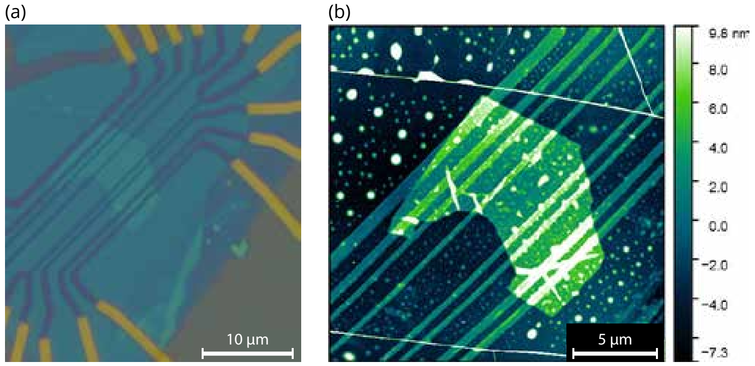


FIG. 1. Images of the final hBN-encapsulated CrBr3/Pt device. (a). An optical microscope image of the device. The contacted $CrBr_3$ flake remains visible through the top encapsulating hBN (b). An Atomic Force Microscopy (AFM) image of the device after fabrication.

The schematic view of the van der Waals structure in Fig.1a in the main text simplifies the device measured, an optical image of the actual device is given in Fig.1a toghether with an Atomic Force Microscopy (AFM) image in Fig.1b.

# III. Magnetic Circular Dichroism measurement

To characterize the magnetic properties of our $CrBr_3$ flakes, we encapsulated a 20 nm-thick $CrBr_3$ flakebetween two wide hBN flakes to form a protected stack dedicated to magnetic circular dichroism (MCD) measurements. Despite the setup was not designed to analyse out-of-plane easy axis magnets, a signal has been successfully acquired using a 17°-tilted magnetic field. Interestingly, the shape and coercive field are perfectly matching the results reported by Kim et al. for a similar angle [3], which is consistent with the fact that our crystal has actually been produced in the same batch as this work.

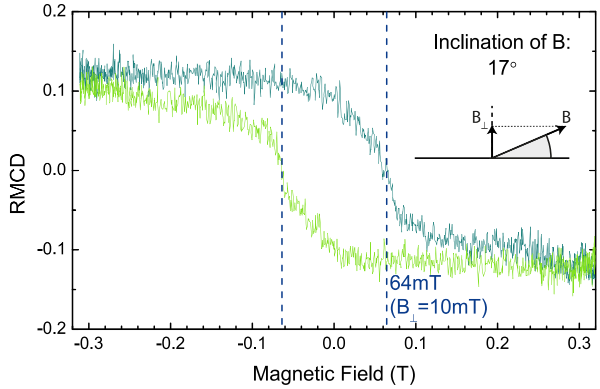


FIG. 2. Reflected Magnetic Circular Dichroism signal measured from a 20nm-thick $CrBr_3$ at low temperature. The measurement setup allowed to incline the magnetic field direction by only 17° from the plane, limiting the actual out-of-plane component. The narrow but clear magnetic hysteresis is reproducible and can indicate a switch of the out-of-plane component of the magnetization at as low as 18.7 mT.

## IV. Electrical measurement

### A. Electrical characterization

The sample is electrically characterized by lock-in amplifiers in low frequency (6Hz to 13Hz). Amplification factor is tested with a 10 kΩ resistor (close to contact resistance). In second harmonic measurement, we extract the -Y component as the second harmonic voltage with phase set to zero in the reference signal.

### B. Local signal

We also measured the local first harmonics and local second harmonics (same contact as the injector and detector), we find no clear signature for Spin Hall Magnetoresistance and local Spin Seebeck Effect. The fitted amplitude of $R_{\mathrm{nl}}^{1\omega}$ is not higher than the noise level, with the maximum sensitivity of the measurement setup.

### C. Non-local first harmonic signals

There are three reasons why we are not able to observe the electrical magnon injection and detection in the first harmonic signal. 1. It requires two inefficient conversions of Spin Hall Effect (SHE) and Inverse Spin Hall Effect (ISHE), while only ISHE is enough for the detection of Spin Seebeck Effect (SSE). 2. Magnons need to travel through a distance of a few hundred nanometers from injector to the detector for the first harmonic signal, while magnons related to the Spin Seebeck effect can be generated closer to the detector. It could be that the magnon relaxation length is shorter than the contact distance in our devices, and electrically generated magnons are therefore not detectable. 3. The range of applied current is limited because a too high Joule heating in the injector region alters the magnetic properties of the layer. As the electrical magnons are generated only under the injection interface, they vanish faster than the thermal magnons still generated far from this region.

### D. Offset of the non-local second harmonics

We observed an offset always presents for the fitted cosine function in the non-local second harmonic measurements. However, The offset varies with current in independent ways for the same measurement on different pairs, as shown in Fig4b.

### E. Methods for nl-ADMR measurements and their fitting

Due to a limited rotation range of our sample holder, we can not finish 360° rotation in one measurement. For all the figures of the main text, data are measured for a positive magnetic field over a 180° range and concatenated to measurement of the same angular range with the opposite magnetic field, physically equivalent to a full cycle of 360°.

All the curve fittings of the angular dependencies are independent fitting of a cosine or sine function (with imposed 0° phase) plus an offset, the amplitude $R_{\mathrm{nl}}^{2\omega}$ and the background level $R_0^{2\omega}$ are respectively the fitted amplitude and offset extracted from this procedure. The error bar is the standard error of the data from a fitted curve.

| Contacts | Width | Spacing to next right contact | Model name |
|---|---|---|---|
| 2-19 | 0.31 $\mu$m | 0.50 $\mu$m | N.A. |
| 6-18 | 0.31 $\mu$m | 2.43 $\mu$m | $w_{Det4}$ |
| 7-15 | 0.31 $\mu$m | 1.24 $\mu$m | $w_{Det3}$ |
| 11-14 | 0.31 $\mu$m | 0.50 $\mu$m | $w_{inj}$ |
| 12-13 | 0.52 $\mu$m | 0.87 $\mu$m | $w_{Det1}$ |
| Unused | 0.73 $\mu$m | N.A. | $w_{Det2}$ |

TABLE I. Width and edge-to-edge spacing for the contacts used in this work. The last column reports the corresponding parameter name used in the simulation. The last contact of the table couldn't be measured but is included in the modeling.

In Fig2 of the main text, the second order nlADMR measured at 60 µA and 80 µA, the angular modulation of the second harmonics is plotted in Fig3. The angular modulation of the second harmonics still exists but it does not follow the shape of SSE and pANE$_z$.

The data was measured in different cool-downs and therefore there could be some changes of the thermal conductivity at the interface between Pt and CrBr3. This can add some variations on the spin-caloritronic signal, as the environment for thermal conduction was changed. For example, data in Fig.2(a)(top) and Fig.1(e) differ by 25%.

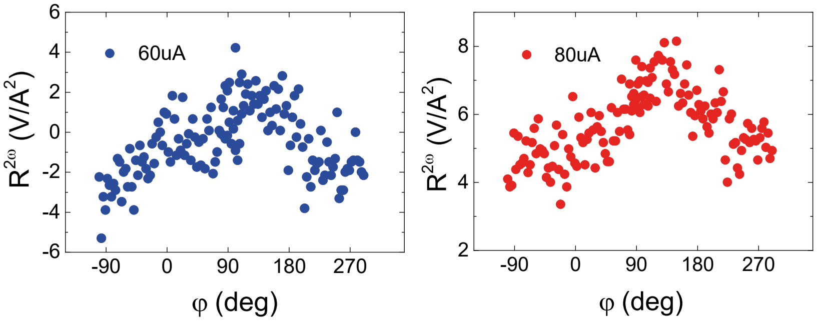


FIG. 3. Supplementary data for Fig.2 of the main text. $R^{2\omega}$ measured at 60 µA and 80 µA, under magnetic field of 4T at 5K.

## V. Spin signal measured at different contact pairs

The second order IP-nlADMR is reproducible and also found in 4 different pairs of contacts (four out of four contacts which are electrically conductive). We plotted, in Fig4c, the amplitudes $R^{2\omega}_{\rm nl}$ extracted from these nlADMR signals as a function of the distance separating the heater electrode from the detector electrode, for four characteristic currents from the range used in this work. Out of these data, though, one cannot observe any clear distance dependence for this signal, for the reasonable current range we applied. Several aspects can be invoked to explain this observation: We have argued that the signal is mostly composed of the sum of SSE induced ISHE, and of pANEz appearing due an out-of-plane temperature gradient in the proximity magnetized Pt. The variation of these two effect, with the different temperature gradients involved, can be complex here. In addition, as mentioned in the main text, the Pt/$CrBr_3$ interface might different for each contact. A few parameter can play roles here, e.g. different effective contact area, different thermal conductivity at the interface and etc. The sign reversal of the IP-nlADMR signal is also reproducible for different pairs of contacts. In Fig4b, examples are shown for 3 different electrical connections.

## VI. Temperature dependence of spin Seebeck signal

Raw data of spin Seebeck signal temperature dependence is plotted in Fig5 (a) and (b). We notice a abnormal high noise level in certain ranges (for example at 0° and 180°) for the sample rotation, as shown in 5 (a) and (b). For the small fitted value of $R^{2\omega}_{\rm nl}$ at 60K, we attribute it to instrumental defects because it is also present in other samples from our colleagues for different projects during the time period when we measured our sample.

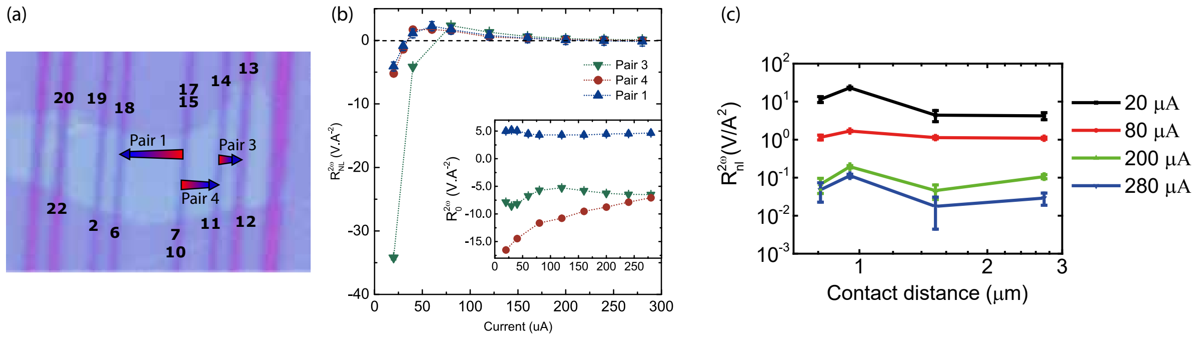


FIG. 4. Current dependence for different pairs. For reference, Pair 3 is the one discussed along the main text. (a) Denomination of contact pairs, the red side indicates the heater contact, the blue side points to the detector contact. (b) Current dependence of the amplitude $R_{\rm nl}^{2\omega}$ second order IP-nlADMR, and in inset, current dependence of the offset $R_0^{2\omega}$ for three contact pairs. (c) Distance dependence of spin Seebeck resistance in log10 scale.

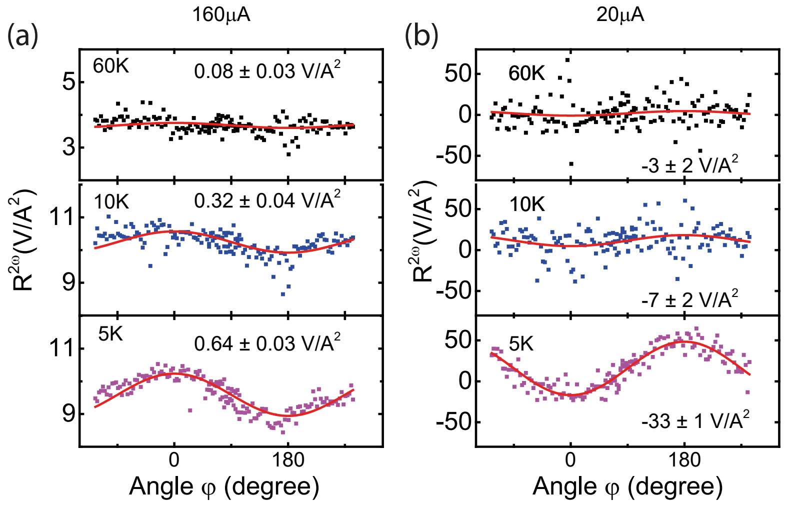


FIG. 5. Temperature dependence raw data.

## VII. Finite element heat distribution simulation

As mentioned in the main text, the encapsulation of $CrBr_3$ into hBN layers leads to multiple heat transfer channels in the system and therefore to a non-trivial variation of in-plane and out-of-plane temperature gradient depending on the heating current. Therefore we propose to qualitatively study the temperature distribution in $CrBr_3$/hBN heterostructure.

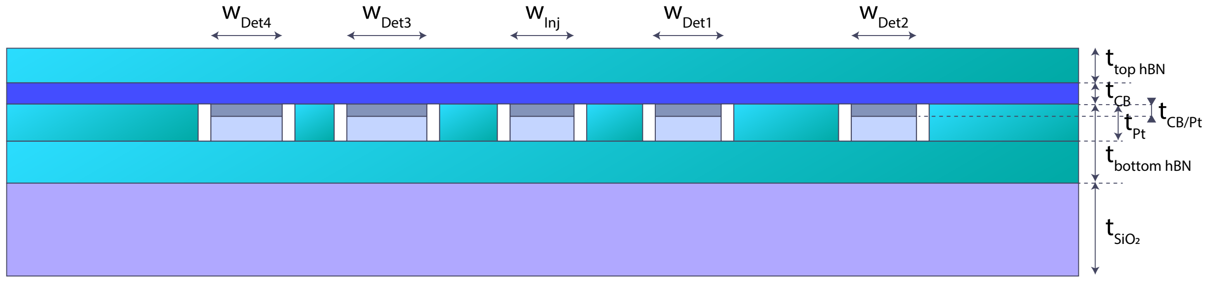


FIG. 6. Schematic of the sample geometry for the simulation.

| Parameter name | Symbol | Value | Source |
|---|---|---|---|
| Platinum thermal conductivity | $\kappa_{\rm Pt}^{\rm 20K}$ | $\gtrsim 475{\rm Wm^{-1}K^{-1}}$ | Database in Ref.[7]; [8] |
| Electrical conductivity | $\sigma_{\rm Pt}^{\rm 5K}$ | $\approx 1.36\times10^{6}\ \Omega^{-1}$ | Measured at 5K |
| Seebeck coefficient | $S_{\rm Pt}^{\rm 5K}$ | $\geq +5\mu{\rm V/K}$ | From Ref.[9] |
| Spin Hall angle | $\Theta_{\rm SH}$ | $\approx 0.05$ | Pessimistic guess from Ref.[10] |
| hBN thermal conductivity | $\kappa_{\rm hBN}^{5-50K}$ | $3-100{\rm Wm^{-1}K^{-1}}$ | Ref.[5] |
| hBN th. Cond. anisotropy | $\kappa_{\rm hBN}^{xy}/\kappa_{\rm hBN}^{xx}$ | $0.002-0.1$ | Parameter, range assessed from [11] |
| CrBr3/Pt interface thermal conductance | $\kappa_{\rm int}^{\rm CrBr_3/Pt}$ | $7\times10^{6}{\rm Wm^{-2}K^{-1}}$ | Estimated from Ref.[6] |

TABLE II. Main parameters and values used for the simulation, and references.

### A. Geometry, conditions and parameters

The two-dimensional model is defined as a slice in the $x$-$z$ plane of the device centrered in the $CrBr_3$ channel, with a geometry and dimensions as close as possible to the real one. We assume a perfectly homogeneous contact between all the layers as defined in Fig.6. In this model the interface between Pt and $CrBr_3$ is defined as a layer with finite small thickness (1 nm). We consider only the thermal diffusion via thermal bulk and interfacial conduction properties of all the materials. The model consists in 5 contacts with our central injector and 2 detectors each side, all with the dimensions as measured by AFM on the actual sample. The pair of contacts we focused on, in the main text, are the central injector and the first detector on the right of it.

In this geometry, we also include a 2nm-spacing between the platinum electrode and the neighboring hBN slab to take into account that the $CrBr_3$ layer is deposited on contacts higher than the hBN surface, then we necessarily have a small empty space between the bent $CrBr_3$ layer, the platinum and the hBN surface. A boundary condition imposes the bottom edge of the silicon oxide layer to be at 5K constantly to account for the thermal contact with the chip carrier maintained at 5K in a VTI, the other edges are left in contact to vacuum as the pressure in the VTI remains below 1 atm.

The thermal conductivity of Platinum can be found down to 20 K in the literature and the electrical conductivity estimated from the measurements in the local signals is also consistent with previous studies. The spin Hall angle of Platinum and its variation in temperature has also been studied and will be considered constant over the temperature range of this study[4]. For the E-beam evaporated platinum that was used here, we consider $\Theta_{SH} = 0.05$. (It can also be noteworthy that the Seebeck coefficient of platinum changes sign between 150 and 200K but this is far beyond the temperature range actually expected in our measurements).

The thermal conductivity of the hBN can be found in the literature for thick layers and low temperature, we include this parameter as temperature dependent by subtracting the results of ref. [5]. 2D layered materials, by nature possess different in-plane and cross-plane interactions, therefore an anisotropy of their properties can be expected. We take into account an anisotropy of the thermal conductivity for hBN introducing an anisotropy factor as $f_{\rm ani} = \kappa_{\rm hBN}^{xy}/\kappa_{\rm hBN}^{xx}$ varied between 0.002 and 0.1 as assessed by reports on graphene and hBN systems, with 0.002 suggested to be more realistic for few-layers thicknesses. As the thermal conductivity of $CrBr_3$ is unknown, we assume for simplicity the same temperature dependence as for hBN but with a multiplicative parameter $\eta_{\rm K} = \kappa^{\rm CrBr_3}/\kappa^{\rm hBN}$. The interfacial conductivities can be approximated by the one of graphene on various materials reported in the review from Sadeghi et al. [6]. In particular, the results from 3nm-FLG/SiO2 extrapolated at 5K would lay around $1\times10^{7}Wm^{-2}K^{-1}$ while for diamond/Au the values would be about $7\times10^{6}Wm^{-2}K^{-1}$. Here after we use the most pessimistic value of $\kappa_{\rm int}^{CrBr3/Pt} \approx 7\times10^{6}Wm^{-2}K^{-1}$ for the interfacial thermal conductances. The parameters used hereafter are summerized in the table II.

### B. Simulation and results

To simulate the system, we use the finite elements software package COMSOL, in which we implement in the case of an anisotropic thermal diffusion with :

$$\nabla\cdot(c\nabla T) = \hat{f}, \text{with } c = \begin{pmatrix}\kappa_{xx} & 0\\ 0 & \kappa_{xy}\end{pmatrix} \text{ and } \hat{f} = \frac{J_c^2}{\sigma} \quad (1)$$

$\hat{f}$ is the source term of Joule heating in the injector, it is set to 0 everywhere else. We run the simulation for ratio $\eta_{\rm K} = \kappa_{\rm CrBr_3}/\kappa_{\rm hBN}$ ranging from 0.01 to 100 (1000 and 5000 too but not physically relevant) and applied currents from 1 μA to 5 mA.

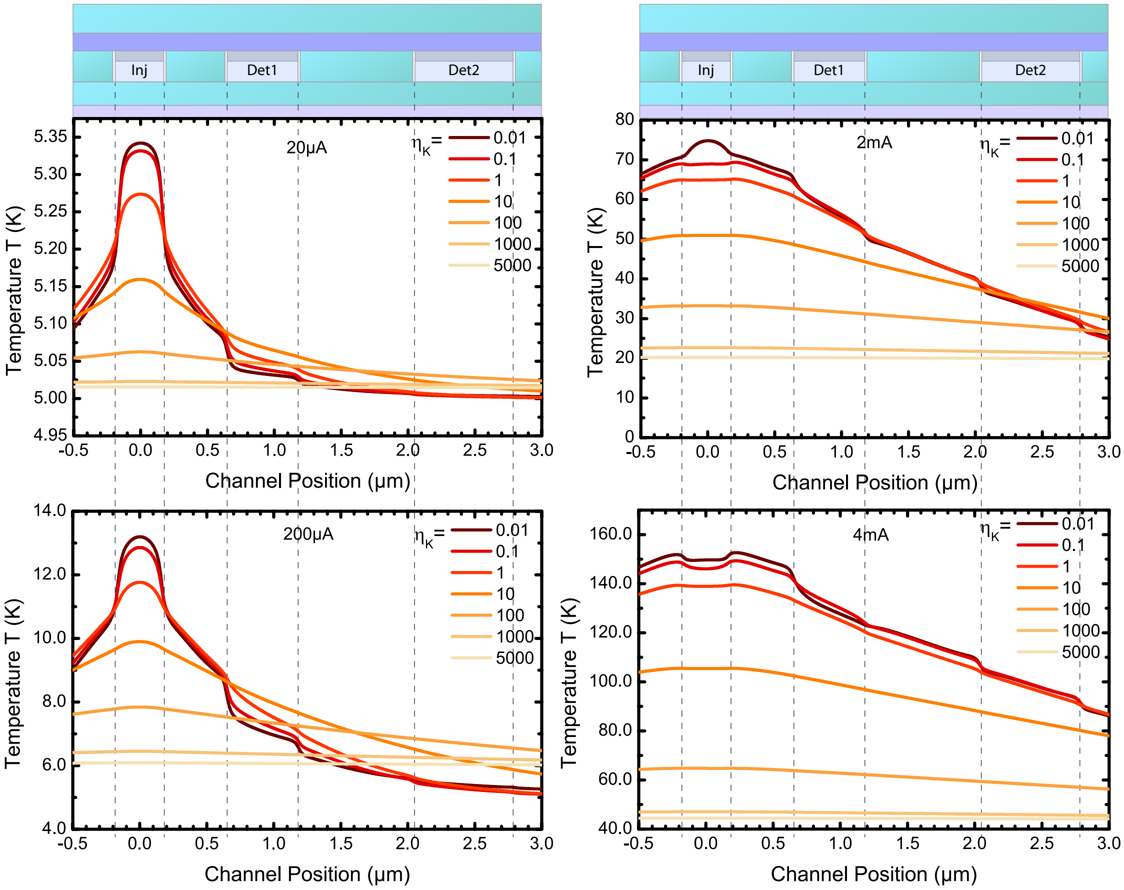


FIG. 7. Profiles of temperature along a line cut at 1 nm above the contacts, into the $CrBr_3$ channel, for 4 currents chosen over the whole range simulated.

### 1. *Temperature profiles in the $CrBr_3$ layer*

On Fig.7, we gather the temperature profiles at 1 nm on top of the platinum contact, into the channel. We show 4 panels, each corresponding to a different heating current applied and each curve shows the profile for a different value of $\eta_K = \kappa_{CrBr_3}/\kappa_{hBN}$.

At 20 μA, we observe that the temperature increase on top of the heater contact is minor, and at most 0.3 K for the lowest thermal conduction of $CrBr_3$. However, this temperature increase becomes rapidely significant while increasing the current. As we don't consider $\eta_K$=1000, 5000 as physically relevant, at 200 μA the temperature already ranges between 10 K and 13 K i.e. between $T_c/4$ and $T_c/3$, while the temperature near the detector stays below 9 K. This supports the approach of taking into account a spatially inhomogeneous thermal conduction parameters. Increasing the temperature furthermore (2 mA, 4 mA) can lead to a local loss of the magnetic ordering by exceeding the Curie temperature $T_c$ on top of the heater only or in the whole device depending on the relative value of the thermal conduction of $CrBr_3$ compared to the one of hBN.

Due to the limited dimensionality of the simulation, two shortcomings are identified:

- The parallel lateral heat paths via the hBN at both sides of the $CrBr_3$ can lead to additional heat exchange inward or outward the $CrBr_3$, which must be a minor correction, and to additional, and most likely asymetric between the two sides, heat exchange with the detector electrode enabling lateral Seebeck effect.
- The actual Pt contact are connected to Au/Ti leads which are themselves laying on the SiO2 substrate. This is a minor but additional heat path from the simulated slice towards the substrate, that can increase slightly the temperature gradients in $z$ axis in the Pt.

From these shortcomings, we expect the axis of currents to be stretched out compared to the reality, and we refer to it mostly qualitatively. With these profiles, we confirm that the thermal confinement of $CrBr_3$ induces a very efficient heating likely to affect its magnetic properties. Therefore, it is obvious that if any magnon phenomena (e.g. SSE, magnon transport,...) from in the channel of $CrBr_3$ can exist, it should rather be expected in the low current regime.

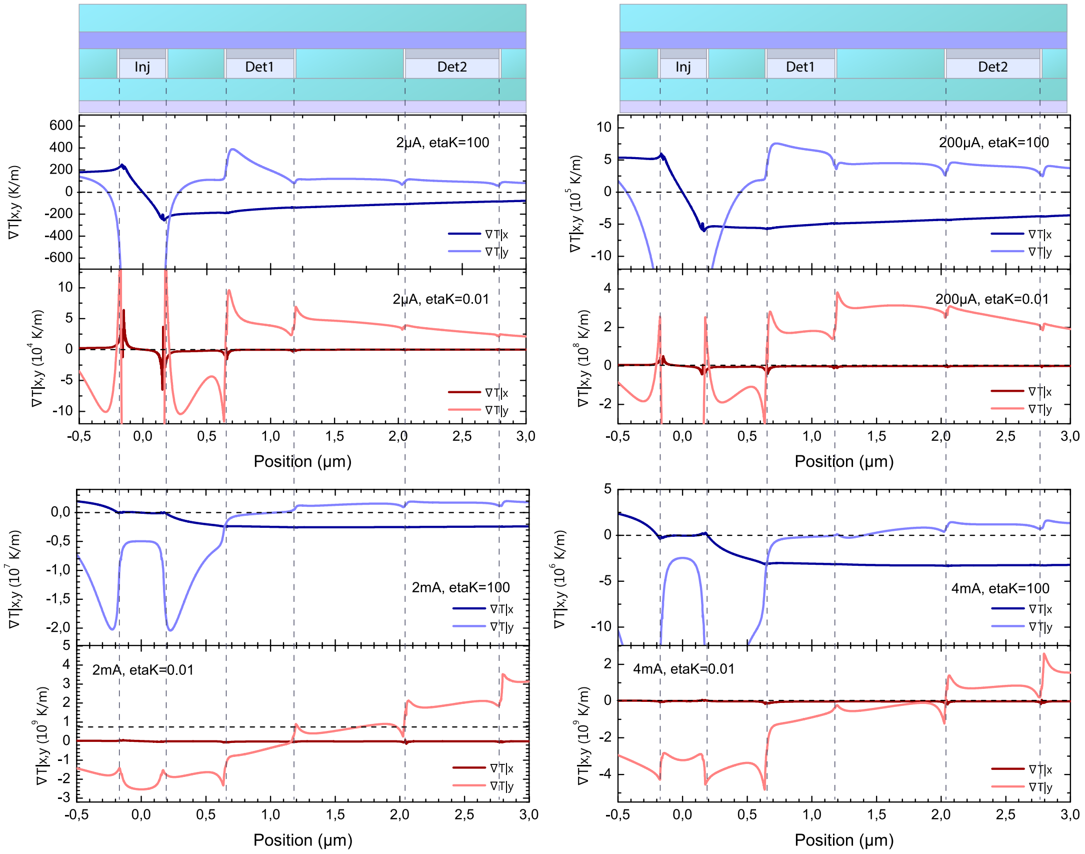


FIG. 8. Profiles of temperature gradients along a line cut at 1 nm above the contacts, into the $CrBr_3$ channel.

### 2. *Temperature gradients profiles in the $CrBr_3$ layer*

The temperature gradient profiles in the $CrBr_3$ layer are given in Fig.8 for the same currents as Fig.7 and in the situation where $\kappa_{\mathrm{CrBr_3}} > \kappa_{\mathrm{hBN}}$ ($\eta_{\mathrm{K}} \gg 1$), and the opposite where $\kappa_{\mathrm{CrBr_3}} < \kappa_{\mathrm{hBN}}$ ($\eta_{\mathrm{K}} \ll 1$). Some observations are noteworthy:

- We first observe that, in either situation of $\eta_{\mathrm{K}}$, $\partial T/\partial z$ reverses its sign between 200 µA and 2 mA, inducing the reversal of any related Longitudinal SSE (if detectable).
- For $\eta_{\mathrm{K}} \ll 1$, the vertical temperature gradient $\partial T/\partial z$ is largely dominating everywhere over the $CrBr_3$ layer and for all currents, and the horizontal gradient $\partial T/\partial x$ is almost non existant except close to the sign reversal point of $\partial T/\partial z$. Therefore any magnon-spin signal measured at the detectors must be dominated by local longitudinal spin Seebeck effect.
- For $\eta_{\mathrm{K}} \gg 1$, the vertical and horizontal temperature gradients can become comparable in the channel, the situation is more complex. At low current (2 µA and 200 µA), right under the *Det1*, we notice $\partial T/\partial x \lesssim \partial T/\partial z$ whereas between the *Inj* and the *Det1* we have $\partial T/\partial x \gg \partial T/\partial z$. The $\partial T/\partial x$ in the inter-contacts region induces a transverse SSE accumulating magnons under the *Det1*, this accumulation added to the one created by the SSE from $\partial T/\partial z$ directly under *Det1* will contribute to the spin-signal in Det1. At high current, though, we observe the opposite situation where $\partial T/\partial x \ll \partial T/\partial z$ between the *Inj* and the *Det1* and $\partial T/\partial x \gg \partial T/\partial z$ under the *Det1*. This can be read as: if there is transverse SSE, it arises closer to *Det1* and only little contribution from a longitudinal SSE (from $\partial T/\partial z$) under the *Det1* to the total magnon-spin signal will be detected.

Once more, all prudence is necessary here considering all the guessed parameters, and until further improvement only qualitative results are used. In addition, the deductions about magnon-spin detection are only indicative as the temperature dependence of the magnetic properties is not included in this model. However, to summarize, in the case of highly thermally conductive $CrBr_3$ and low heating current, the spin signal measured can be a mixed contribution from local spin Seebeck effect and detection of diffused magnons generated in the bulk channel. We cannot disentangle this situation from a purely interfacial SSE with solely the present data but a clearer answer can be given by measuring the thermal conductivity of CrBr3 at low temperature.

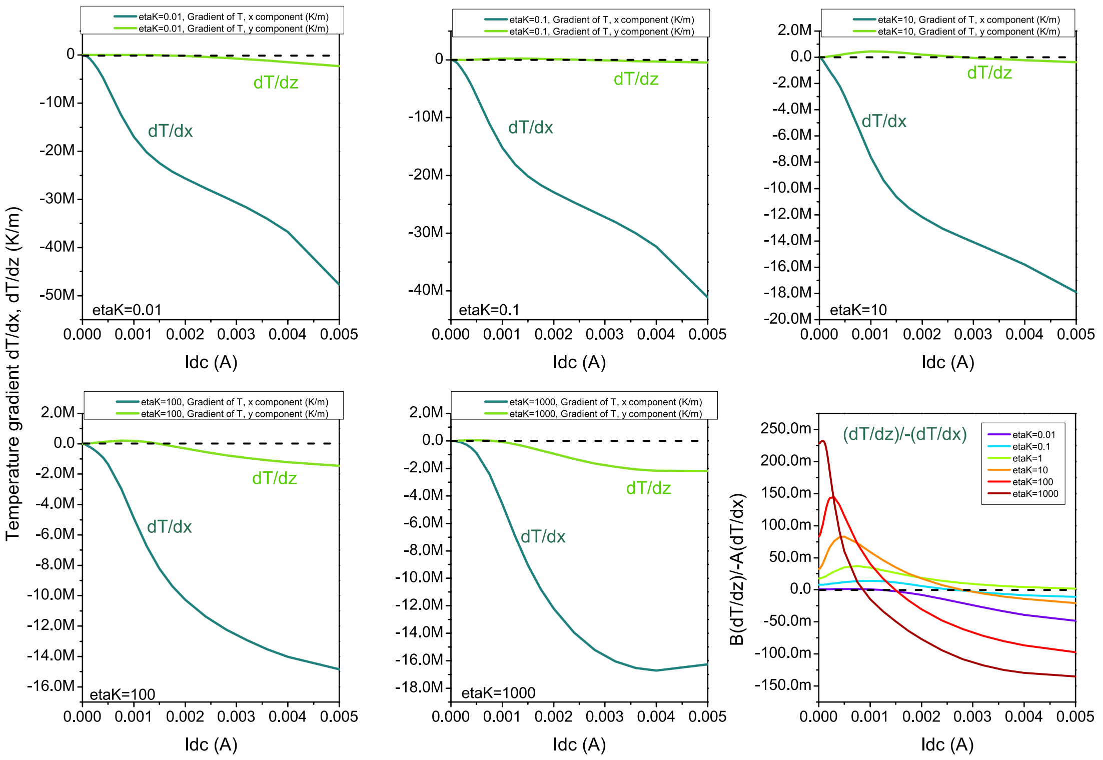


FIG. 9. Current dependence of the averaged temperature gradients along the $x$ and $z$ axes in the platinum detector 1.

### 3. *Temperature gradients in the platinum detector and at the interface*

The current dependence of the average temperature gradients $\langle \partial T/\partial x\rangle_{\mathrm{Pt}}$ and $\langle \partial T/\partial z\rangle_{\mathrm{Pt}}$ into the platinum detector *Det1* (simply written as $\partial T/\partial x$ and $\partial T/\partial z$ in the main text) are given in Fig.9. The $\xi = -R_{\mathrm{SSE+pANE}_z}/R_{\mathrm{pANE}_x}$ mentioned in the main text is shown in the last panel. As $\partial T/\partial x$ doesn't change sign, plotting $\xi$ highlights the sign reversal of $\partial T/\partial z$ with varying the current. The further from $\eta_{\mathrm{K}} = 1$, the lower current is needed for the sign reversal, and this reversal point goes even faster towards the low currents for $\eta_{\mathrm{K}} \gg 1$. Most importantly, for every case we have clearly $\langle \partial T/\partial x\rangle_{\mathrm{Pt}} > \langle \partial T/\partial z\rangle_{\mathrm{Pt}}$

We give the current dependence of the temperature difference $T^{\mathrm{CrBr_3}} - T^{\mathrm{Pt}}$ at the interface CrBr$_3$/Pt in Fig.10. This is a check that the sign reversal of $\langle \partial T/\partial z\rangle_{\mathrm{Pt}}$ is concomitant to the sign reversal of the temperature difference at the interface Pt/CrBr$_3$.

## C. Estimation of a spin Seebeck coefficient

To allow for a first estimation of the spin Seebeck coefficient, we assume a the perfect thermalization of the magnon bath with the phonon bath which translates into the approximation $T_{\mathrm{m}}^{\mathrm{CB}} \approx T_{\mathrm{ph}}^{\mathrm{CB}} = T^{\mathrm{CB}}$ and $T_{\mathrm{e}}^{\mathrm{Pt}} \approx T_{\mathrm{ph}}^{\mathrm{Pt}} = T^{\mathrm{Pt}}$. Then the spin current induced by spin Seebeck effect at the interface between Pt and CB gives : $j_s^{\mathrm{int}} \approx L_s \left(T_{\mathrm{m}}^{\mathrm{CB}}|_{\mathrm{int}} - T_{\mathrm{e}}^{\mathrm{Pt}}|_{\mathrm{int}}\right)$ with $L_s = g_s S_s$.

In the main text, our extraction procedure for the SSE contribution suggests that the SSE should contribute the most for low heating currents. According to the extracted data for 20 µA in Fig.4f of the main text, if we take the mean value $R_{\mathrm{nl}}^{2\omega} = -47$ V.A$^{-2}$ i.e., for a contact length of 10.3 µm, an EMF of $E_{\mathrm{ISHE}} = -V_{\mathrm{nl}}^{2\omega}/L = 1.29$ mV.m$^{-1}$. On the simulated current dependences, all the traces show rapid increase, a peak, and a decreasing slope. With regards to our measurements, we can suppose that in our system, at 20 µA, we lay on the beginning of the decreasing slope, so for we use from the model the value for $\eta_{\mathrm{K}} = 10$ at $I = 2mA$ i.e. $T_{\mathrm{m}}^{\mathrm{CrBr_3}} - T_{\mathrm{e}}^{\mathrm{Pt}} = 1.5$ K. This leads to :

$$L_s = \frac{J_s}{T_{\mathrm{m}}^{\mathrm{CrBr_3}} - T_{\mathrm{e}}^{\mathrm{Pt}}} = \frac{E_{\mathrm{ISHE}} \times \sigma_{\mathrm{Pt}}}{\Theta_{SH}\left(T_{\mathrm{m}}^{\mathrm{CrBr_3}} - T_{\mathrm{e}}^{\mathrm{Pt}}\right)} \approx 2.34 \times 10^4 \mathrm{A.K}^{-1} \quad (2)$$

Considering $g_s \leq g_s^{YIG} = 0.16 \times 0.7 \times 10^{14}\,\Omega^{-1}.m^{-2}$, we deduce $S_s = L_s/g_s \geq 2.09$ nV.K$^{-1}$. This value is a lower bound as we made the assumption of a spin mixing conductance equal to the one of Pt/YIG which is the highest

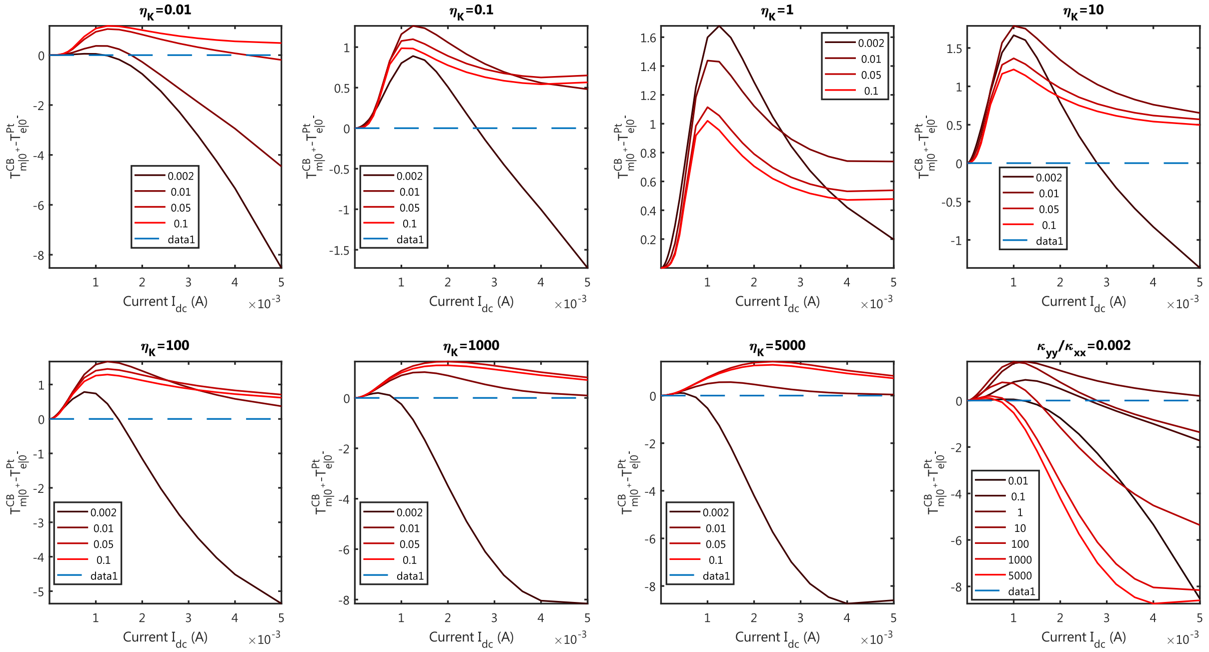


FIG. 10. Heating current dependence of the difference of temperature at the interface Pt/CrBr3. Each of the 7 first panels show the current dependence for a particular $\eta_K = \kappa_{\mathrm{CrBr_3}}/\kappa_{\mathrm{hBN}}$ ratio, for anisotropy factors varying 0.002 to 0.1. The last panel focuses on an anisotropy of 0.002 and shows all the $\eta_K$ values

value known so far. As an example, if we consider $g_s$ two orders of magnitude lower, $g_s = 0.16 \times 0.7 \times 10^{12}\,\Omega^{-1}.m^{-2}$, we get $S_s = L_s/g_s \geq 0.209\mu$ V.K$^{-1}$ closer to the spin Seebeck coefficient generally found.

## VIII. An overview of bulk, interface and proximity spin-caloritronics effects

As the measurements are carried out at low temperature while significantly high currents are passed through the contacts, we expect the presence of non-negligible temperature gradients along the whole device, which is supported by the simulation. Therefore, for completeness, we review here the various magneto-caloritronic effects that have been previously reported in others systems[12] that might arise in our system due to these gradients and in presence of a magnetic field or by proximity effect of platinum with a magnetic material. We discuss their contribution to the measured signal in terms of symmetries and order of magnitude.

### A. Seebeck effect

While probing the voltage drop over the platinum electrode, one can expect the contribution of an additional Seebeck voltage drop in presence of a temperature gradient $\partial_y T$ in the $y$ direction. However, with the geometry of the experiment described in the main text, this temperature gradient can only arise from thermal conductance inhomogeneities and which cannot be avoided due to the irregular shapes of the flakes but this gradient should be largely negligible compared to the longitudinal and vertical gradients. Moreover this contribution is independent of the magnetization direction and shall only contribute to the offset of the second harmonic signal measured.

### B. Spin Nernst Magnetoresistance

The Spin Nernst Magnetoresistance (SNMR) is the analog of the spin Hall Magnetoresistance (SMR) as the spin Nernst effect (SNE), at the origin of it, is the analog of the spin Hall effect at the origin of the SMR [13, 14], where the driving force is a thermal gradient instead of the voltage gradient. The spin current $\vec{J}^{s\,SNE}_{j,k}$ generated can be expressed by the relation:

$$\vec{J}^{\mathrm{s}\;\mathrm{SNE}}_{j,k} = -\frac{\hbar}{2|e|}\Theta_{\mathrm{SN}}\left(\overrightarrow{e_k} \times \frac{S_{\mathrm{Pt}}}{\rho_{\mathrm{Pt}}}(-\vec{\nabla}T)\right)_j \tag{3}$$

Where $j, k \in \{x, y, z\}$ with $j$ the component of the spin current, $k$ is the direction of polarization of the spin and $\vec{e_k}$ the unit vector representing this direction, $\Theta_{\text{SN}}$ is the spin Nernst angle characterizing the charge-to-spin conversion, $S_{\text{Pt}}$ and $\rho_{\text{Pt}}$ are respectively the Seebeck coefficient and the resistivity of the platinum electrode.

Again, as we probe a voltage drop along the $y$ axis, only the SNMR contribution from a temperature gradient along the y axis can be detected, which we expect to be minor, as mentioned in the previous section. Furthermore, the angular dependence of this signal should be the same as SMR: when the polarization $\vec{\sigma}$ of the SNE-induced spin current is aligned with the magnetization $\vec{M}$, the carriers are reflected at the interface and converted back to a charge current by ISHE, inducing a peak of voltage (for $\phi = 0, 180°$), whereas when $\vec{\sigma}$ and $\vec{M}$ are orthogonal, the spin momentum is absorbed by the magnet inducing a spin flip of the electron, hence a ISHE current opposite to the one creating it, and a minimum of voltage (for $\phi = 90, 270°$). The overall angular dependence follows a cosine modulation with 180°period, not consistent with the clear 360°periodicity we measure.

As a result, the measurement geometry allows the presence of a SNMR contribution but not only its magnitude is expected to be small, its specific angular dependence leads us to rule out this effect as the major contribution to the measured second harmonic signal exposed in this study.

## C. Proximity Anomalous Nernst Effect

### *1. Relevance of a proximity induced magnetism in platinum*

Several works question and argue the possibility to magnetize a thin platinum layer in contact with a ferromagnet. The efficient magnetization of a non-magnetic material by proximity exchange coupling with a magnetic material has already been studied theoretically in Cobalt/bilayer hBN on Graphene[15] or measured in Graphene on YIG[16]. In addition, platinum is close to the Stoner criterion, its interplay with ferromagnets has been computed for proximity with YIG[17] and magnetoresistance signals as well as XMCD magnetic moments have been reported confirming a partial magnetization of the platinum layer [18]. Therefore comes for our system the possibility to measure a contribution to the signal not related to magnon transport but to a mgnetized part of the platinum.

### *2. Contribution of the anomalous Nernst effect*

Assuming the Pt can be magnetized in the vicinity of the interface, an Anomalous Nernst voltage generated there would be expressed by:

$$\nabla V_{\text{AN}} = -S_{\text{AN}} \left( \mathbf{m} \times [-\nabla T] \right) \tag{4}$$

Where $S_{\text{AN}}$ is Anomalous Nernst coefficient, $\mathbf{m}$ is the unit vector representing the direction of the induced magnetization.

If we assume that the effective magnetization present in the platinum behaves as the magnetization of $CrBr_3$ with regards to the field and we consider the cases where it is saturated and fully following the magnetic field, several configurations lead to a contribution of this effect in our measurements.

In the case of the magnetization rotated in-plane:

- If we consider whatever in-plane temperature gradient ($\partial_x T$, $\partial_y T \neq 0$), $\left(\vec{m} \times (-\vec{\nabla} T)\right)$ still has no component along the $y$ axis and therefore cannot contribute to our measured voltage. The case $\partial_y T \neq 0$, only the Seebeck voltage might add up to the signal as explained earlier.
- If we consider the out-of-plane temperature gradient pointing to positive $z$ ($-\partial_z T < 0$): $\Delta V_y^{\text{ANE}} \propto \left(\vec{m} \times (-\vec{\nabla} T)\right)_y$ cancels out for $\phi = -90, 90°$ and $\left(\vec{m} \times (-\vec{\nabla} T)\right)_y$ gives a negative contribution for $\phi = 0°$ and positive contribution for $\phi = 180°$. The angular dependence here follows a cosine function of the angle $\phi$. This obviously leads to a 360° periodicity, and the same angular dependence as the SSE signal expected.

For the out-of-plane rotation of the magnetization:

- If we consider the in-plane temperature gradient pointing to negative $x$ ($-\partial_x T > 0$): $\Delta V_y^{\text{ANE}} \propto \left(\vec{m} \times (-\vec{\nabla} T)\right)_y$ cancels out for $\theta = 0, 180°$, but gives a positive contribution for $\theta = 90°$ and a negative contribution for $\theta = -90°$. The angular dependence then obeys a sine function of the angle $\theta$.

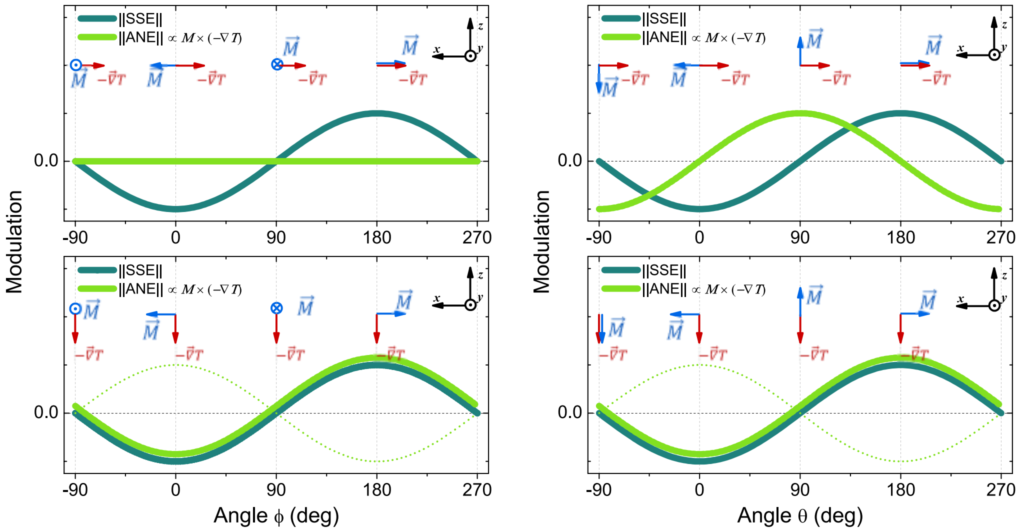


FIG. 11. Schematic representation of the expected angular dependence of the ANE for in-plane (b) and out-of-plane (a) magnetic field rotation. This description holds when assuming the magnetization in Pt is saturated by the applied magnetic field at 4T.

- Finally if we consider the out-of-plane temperature gradient pointing to positive $z$ ($-\partial_z T < 0$): the result is the same as for the in-plane rotation. We operate a $-90°$ rotation around the $y$ axis: $\Delta V_y^{\mathrm{ANE}} \propto \left(\vec{m} \times (-\vec{\nabla} T)\right)_j$ cancels out for $\theta = -90, 90°$ and $\left(\vec{m} \times (-\vec{\nabla} T)\right)_j$ gives a negative contribution for $\theta = 0°$ and positive contribution for $\theta = 180°$. The angular dependence here follows a cosine function of the angle $\theta$.

### 3. *Revealing the anomalous Nernst effect induced by horizontal heat flow*

As we identified a different angular dependence of the pANE contribution due to $-\partial_x T$, when reversing the heater and detector contacts, thus reversing the sign of $-\partial_x T$, according to Eq.4, the contribution due to $\partial_x T$ (pANE$_x$) is expected to reverse its sign, whereas the contribution due to $\partial_z T$ (pANE$_z$) will conserve its sign. For clarity, we can describe the two signals in term of normalized resistance $\rho_i = R^{2\omega} S^i_{\mathrm{Pt}}/L^i_{\mathrm{Pt}}$, with $S^i_{\mathrm{Pt}}$ the cross-section and $L^i_{\mathrm{Pt}}$ the length of the detection electrode for the configuration $i$. For the forward (F) and reverse (R) configurations, the signal can be expressed as:

$$\begin{aligned} \rho_{\mathrm{F}} &= y_{\mathrm{F}} + A_{\mathrm{F}}\ cos\theta + B_{\mathrm{F}}\ sin\theta \\ \rho_{\mathrm{R}} &= y_{\mathrm{R}} + (1+\alpha)\, A_{\mathrm{F}}\ cos\theta - (1+\beta)\, B_{\mathrm{F}}\ sin\theta \end{aligned} \tag{5}$$

With $\alpha,\ \beta \approx 0$ being some asymmetry factors accounting for the slight difference of thermal power produced by different heater contacts in the two configurations as well as the anisoropy of the anomalous Nernst coefficient $S_{\mathrm{AN}}$. To verify the presence of these effects, adding up the *forward* and *reversed* configuration measurements will give the ANE$_x$ and cancel out pANE$_z$, subtracting them will give pANE$_z$ and cancel out pANE$_x$:

$$\begin{aligned} \rho_{(\mathrm{SSE+pANE}z)} &= \frac{\rho_{\mathrm{F}} + \rho_{\mathrm{R}}}{2} = \frac{y_F + y_{\mathrm{R}}}{2} + \left(1 + \frac{\alpha}{2}\right) A_{\mathrm{F}}\ cos\theta - \frac{\beta}{2} B_{\mathrm{F}}\ sin\theta \\ \rho_{\mathrm{pANE}x} &= \frac{\rho_{\mathrm{F}} - \rho_{\mathrm{R}}}{2} = \frac{y_F - y_{\mathrm{R}}}{2} - \frac{\alpha}{2} A_{\mathrm{F}}\ cos\theta + \left(1 + \frac{\beta}{2}\right) B_{\mathrm{F}}\ sin\theta \end{aligned} \tag{6}$$

Assuming $\alpha,\ \beta = 0$:

$$\begin{aligned} \rho_{(\mathrm{SSE+pANE}z)} &= \frac{\rho_{\mathrm{F}} + \rho_{\mathrm{R}}}{2} = \frac{y_{\mathrm{F}} + y_{\mathrm{R}}}{2} + A_{\mathrm{F}}\ cos\theta \\ \rho_{\mathrm{pANE}x} &= \frac{\rho_{\mathrm{F}} - \rho_{\mathrm{R}}}{2} = \frac{y_{\mathrm{F}} - y_{\mathrm{R}}}{2} + B_{\mathrm{F}}\ sin\theta \end{aligned} \tag{7}$$

The result of these operations is shown in Fig.4c in the main text for an applied field of 4T and current of 20 $\mu$A, along with the fitting of SSE+pANE$_z$ and pANE$_x$ signals respectively with cosine and sine functions. As a result we

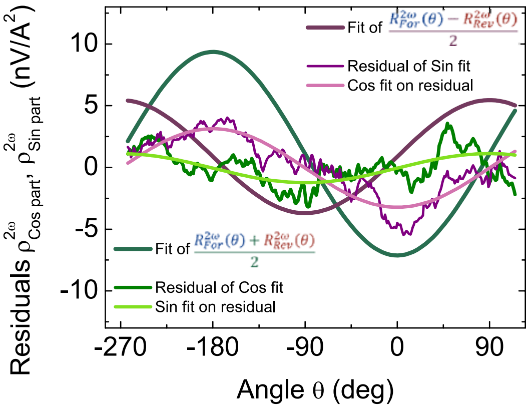


FIG. 12. Extraction of the power asymmetry factors. Result of the summation (Light green) and subtraction (Light purple) of the two configurations. The thick green (purple) line reproduces the cosine (sine) fit of Fig.4c of the main text, the thin green (purple) line is the residual curve of this fit, the light green (pink) curve is the sine (cosine) fit of the residual corresponding to non-zero $\alpha$ and $\beta$ in Eq.5. We obtain $\alpha = -0.77$ and $\beta = -0.51$.

get an offset $y_{\text{F}} \approx y_{\text{R}} \approx 1.1 \pm 0.08$ nV.m.A$^{-2}$, and the amplitudes $A_{\text{F}} = -8.25 \pm 0.10$ nV.m.A$^{-2}$ and $B_{\text{F}} = 4.58 \pm 0.17$ nV.m.A$^{-2}$. The discrepancy between the data and fittings can be easily explained by the fact we assumed a perfectly identical power dissipation between the configurations ($\alpha = \beta = 0$) which is an approximation. For completeness, we can extract the power asymmetry factor $\alpha$ and $\beta$ by fitting their respective contribution into the residuals of the previous fit (so sine function for $\alpha$ and cosine for $\beta$ ) as shown on Fig.12.

### D. Extraction of the spin Seebeck contribution

$$
\begin{aligned}
\nabla V_{\text{AN}} &= -S_{\text{AN}} \begin{pmatrix} m_x \\ m_y \\ m_z \end{pmatrix} \times - \begin{pmatrix} \partial_x T \\ \partial_y T \\ \partial_z T \end{pmatrix} \\
\nabla V_{\text{AN}} &= S_{\text{AN}} \begin{pmatrix} \cos\theta\cos\varphi \\ \cos\theta\sin\varphi \\ \sin\theta \end{pmatrix} \times \begin{pmatrix} \partial_x T \\ \partial_y T \\ \partial_z T \end{pmatrix} \\
\nabla V_{\text{AN}} &= S_{\text{AN}} \begin{pmatrix} \cos\theta\sin\varphi\partial_z T - \sin\theta\partial_y T \\ \sin\theta\partial_x T - \cos\theta\cos\varphi\partial_z T \\ \cos\theta\cos\varphi\partial_y T - \cos\theta\sin\varphi\partial_x T \end{pmatrix}
\end{aligned}
\tag{8}
$$

Then for the in-plane configuration ($\theta = 0, \partial_y T = 0$):

$$
\frac{\Delta V_{\text{AN}}}{L_{\text{Pt}}} \mathbf{u_y} = -S^{\varphi}_{\text{AN}} cos\varphi \partial_z T \mathbf{u_y} \tag{9}
$$

Then for the out-of-plane configuration ($\varphi = 0, \partial_y T = 0$):

$$
\frac{\Delta V_{\text{AN}}}{L_{\text{Pt}}} \mathbf{u_y} = S^{\theta}_{\text{AN}} \left( sin\theta \partial_x T - cos\theta \partial_z T \right) \mathbf{u_y} \tag{10}
$$

According to Eq.4, for $\theta = 90°$, $\Delta V_{\text{AN}} = L_{\text{Pt}} \nabla V_{\text{AN}}$ results in a positive voltage, consistent with $B_{\text{F}} = 4.58\, nV.A^{-2} > 0$ extracted in the previous section. Even if the coefficient $S_{\text{AN}}$ is not strictly the same for ANE$_x$ and ANE$_z$, we can assume it keeps the same sign. Also from the angular dependence sketched in Fig.11, the pANE$_z$ signal is of same sign as the expected SSE. It is therefore relevant to get an order of magnitude of the pANE voltage we can expect, and evaluate its contribution to the total signal.

In addition, and to be precise, the pANE voltage must be re-normalized by a factor $\left( \frac{t^I_{\text{Pt}}}{t_{\text{Pt}}} \right)$ taking into account the shunt that the non-magnetic region of the Pt electrode applies over its thin magnetized region, as adapted from Kikkawa et al.[19] (Fig.13a). This can be expressed as effective anomalous Nernst coefficients :

$$
S^{\text{x,eff}}_{\text{AN}} = \left( \frac{t^I_{\text{Pt}}}{t_{\text{Pt}}} \right) S^x_{\text{AN}};\ S^{\text{z,eff}}_{\text{AN}} = \left( \frac{t^I_{\text{Pt}}}{t_{\text{Pt}}} \right) S^z_{\text{AN}} \tag{11}
$$

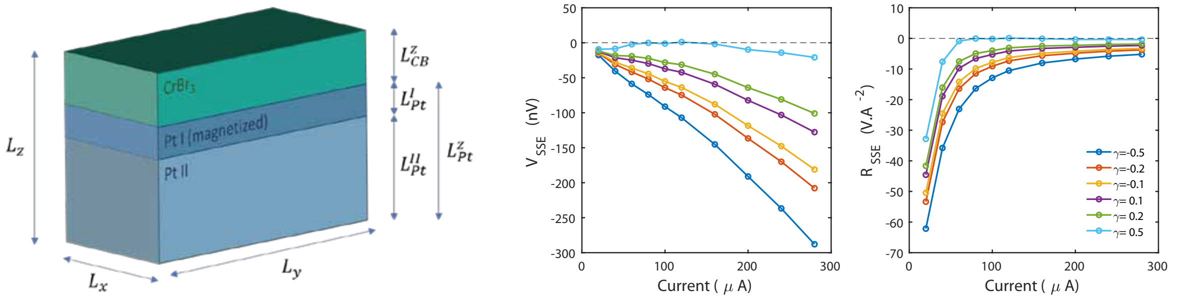


FIG. 13. Schematic of the 2-layer platinum system to describe the shunting effect, adapted from [19]. Current dependence of the estimated SSE voltage (a) and resistance (b), for a range of $\gamma$ between negligible $\partial_z T$ and $\partial_z T$ comparable to $\partial_x T$. Our model is expected to underestimate $\partial_z T$ so we consider intermediate values of 0.1 to 0.5 as the most relevant.

with $t^I_{\mathrm{Pt}}/t_{\mathrm{Pt}} = 0.18$ ($t_{\mathrm{Pt}} = 5.5\ nm$, $t^I_{\mathrm{Pt}} \approx 1\ nm$). Finally, in out-of-plane nlADMR measurement configuration, the pANE resistance contribution reads:

$$\Delta V_{\mathrm{AN}} = L_{\mathrm{Pt}} \left( S^{\mathrm{x,eff}}_{\mathrm{AN}} \sin\theta \partial_x T - S^{\mathrm{z,eff}}_{\mathrm{AN}} \cos\theta \partial_z T \right) \tag{12}$$

Setting $\gamma = \frac{\partial_z T}{\partial_x T}$ and $\delta = \frac{S^{\mathrm{z,eff}}_{\mathrm{AN}}}{S^{\mathrm{x,eff}}_{\mathrm{AN}}}$, the total $R^{2\omega}$ signal measured can be fitted with the following expression:

$$R^{2\omega} = R_0 + A\cos\theta + B\sin\theta, \text{ where } \begin{cases} A = & R_{\mathrm{SSE}} - \frac{\sqrt{2}L_{\mathrm{Pt}}}{I^2} S^{\mathrm{z,eff}}_{\mathrm{AN}} \partial_z T \\ B = & \frac{\sqrt{2}L_{\mathrm{Pt}}}{I^2} S^{\mathrm{x,eff}}_{\mathrm{AN}} \partial_x T \end{cases} \tag{13}$$

Defining $\xi = \frac{-A}{B}$, we get:

$$\xi = \frac{\left(\frac{\sqrt{2}L_{\mathrm{Pt}}}{I^2}\right) S^{\mathrm{z,eff}}_{\mathrm{AN}} \partial_z T - R_{\mathrm{SSE}}}{\left(\frac{\sqrt{2}L_{\mathrm{Pt}}}{I^2}\right) S^{\mathrm{x,eff}}_{\mathrm{AN}} \partial_x T} = \frac{S^{\mathrm{z,eff}}_{\mathrm{AN}}}{S^{\mathrm{x,eff}}_{\mathrm{AN}}} \frac{\partial_z T}{\partial_x T} - \frac{R_{\mathrm{SSE}}}{B} = \delta\gamma - \frac{R_{\mathrm{SSE}}}{B} \tag{14}$$

Hence:

$$R_{\mathrm{SSE}} = (\delta\gamma - \xi)B \tag{15}$$

As a consequence, the contribution from the SSE in our system can be extracted from the measurement, provided that:

- the $\delta$ ratio of proximity ANE coefficients is close to 1
- the $\gamma$ ratio of temperature gradients is known or, as in this work, evaluated qualitatively in from simulation (Fig. 9), the result is plotted in Fig. 13. $\gamma$ always remains clearly below 1.

With the assumptions detailed above, we reveal the contribution of the SSE to our measured signal as a function of the heating current, as plotted in Fig13.

---


[1] D. Ghazaryan, M. T. Greenaway, Z. Wang, V. H. Guarochico-Moreira, I. J. Vera-Marun, J. Yin, Y. Liao, S. V. Morozov, O. Kristanovski, A. I. Lichtenstein, M. I. Katsnelson, F. Withers, A. Mishchenko, L. Eaves, A. K. Geim, K. S. Novoselov, and A. Misra, Magnon-assisted tunnelling in van der Waals heterostructures based on CrBr3, Nature Electronics **1**, 344 (2018).

[2] P. Zomer, S. Dash, N. Tombros, and B. Van Wees, A transfer technique for high mobility graphene devices on commercially available hexagonal boron nitride, Applied Physics Letters **99**, 232104 (2011).

[3] M. Kim, P. Kumaravadivel, J. Birkbeck, W. Kuang, S. G. Xu, D. G. Hopkinson, J. Knolle, P. A. McClarty, A. I. Berdyugin, M. Ben Shalom, R. V. Gorbachev, S. J. Haigh, S. Liu, J. H. Edgar, K. S. Novoselov, I. V. Grigorieva, and A. K. Geim, Micromagnetometry of two-dimensional ferromagnets, Nature Electronics **2**, 457 (2019).

[4] M. Isasa, E. Villamor, L. E. Hueso, M. Gradhand, and F. Casanova, Temperature dependence of spin diffusion length and spin Hall angle in Au and Pt, Physical Review B **91**, 024402 (2015).

[5] E. K. Sichel, R. E. Miller, M. S. Abrahams, and C. J. Buiocchi, Heat capacity and thermal conductivity of hexagonal pyrolytic boron nitride, Physical Review B **13**, 4607 (1976).
[6] M. M. Sadeghi, M. T. Pettes, and L. Shi, Thermal transport in graphene, Solid State Communications **152**, 1321 (2012).
[7] The PGM Database, Platinum data, `http://www.pgmdatabase.com/jmpgm`.
[8] J. Matthey, *Platinum Metals Review*, edited by J. Matthey, Vol. 28 (Johnson Matthey Public Limited Company, London, 1984) pp. 164–165.
[9] N. Cusack and P. Kendall, The Absolute Scale of Thermoelectric Power at High Temperature, Proceedings of the Physical Society **72**, 898 (1958).
[10] N. Vlietstra, J. Shan, V. Castel, B. J. van Wees, and J. Ben Youssef, Spin-Hall magnetoresistance in platinum on yttrium iron garnet: Dependence on platinum thickness and in-plane/out-of-plane magnetization, Physical Review B **87**, 184421 (2013).
[11] J. D. Renteria, S. Ramirez, H. Malekpour, B. Alonso, A. Centeno, A. Zurutuza, A. I. Cocemasov, D. L. Nika, and A. A. Balandin, Strongly Anisotropic Thermal Conductivity of Free-Standing Reduced Graphene Oxide Films Annealed at High Temperature, Adv. Funct. Mater. **25**, 4664 (2015).
[12] D. Meier, D. Reinhardt, M. van Straaten, C. Klewe, M. Althammer, M. Schreier, S. T. B. Goennenwein, A. Gupta, M. Schmid, C. H. Back, J.-M. Schmalhorst, T. Kuschel, and G. Reiss, Longitudinal spin Seebeck effect contribution in transverse spin Seebeck effect experiments in Pt/YIG and Pt/NFO, Nature Communications **6**, 8211 (2015).
[13] S. Meyer, Y.-T. Chen, S. Wimmer, M. Althammer, T. Wimmer, R. Schlitz, S. Geprägs, H. Huebl, D. Ködderitzsch, H. Ebert, G. E. W. Bauer, R. Gross, and S. T. B. Goennenwein, Observation of the spin Nernst effect, Nat. Mater. **16**, 977 (2017).
[14] D.-J. Kim, C.-Y. Jeon, J.-G. Choi, J. W. Lee, S. Surabhi, J.-R. Jeong, K.-J. Lee, and B.-G. Park, Observation of transverse spin Nernst magnetoresistance induced by thermal spin current in ferromagnet/non-magnet bilayers, Nature Communications **8**, 1400 (2017).
[15] K. Zollner, M. Gmitra, T. Frank, and J. Fabian, Theory of proximity-induced exchange coupling in graphene on hBN/(Co, Ni), Physical Review B **94**, 155441 (2016).
[16] J. C. Leutenantsmeyer, A. A. Kaverzin, M. Wojtaszek, and B. J. van Wees, Proximity induced room temperature ferromagnetism in graphene probed with spin currents, 2D Materials **4**, 014001 (2016).
[17] G. Y. Guo, Q. Niu, and N. Nagaosa, Anomalous Nernst and Hall effects in magnetized platinum and palladium, Physical Review B **89**, 214406 (2014).
[18] Y. M. Lu, Y. Choi, C. M. Ortega, X. M. Cheng, J. W. Cai, S. Y. Huang, L. Sun, and C. L. Chien, Pt Magnetic Polarization on $Y3Fe5O12$ and Magnetotransport Characteristics, Physical Review Letters **110**, 147207 (2013).
[19] T. Kikkawa, K. Uchida, S. Daimon, Y. Shiomi, H. Adachi, Z. Qiu, D. Hou, X.-F. Jin, S. Maekawa, and E. Saitoh, Separation of longitudinal spin Seebeck effect from anomalous Nernst effect: Determination of origin of transverse thermoelectric voltage in metal/insulator junctions, Physical Review B **88**, 214403 (2013).
